# Supplementary material for: List Items One by One: A New Data Source and Learning Paradigm for Multimodal LLMs
Source: arXiv:2404.16375 source file (2025-01-20)

# SoM Granularity

Level - 1

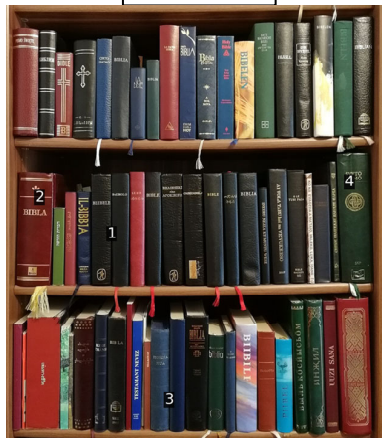

Level - 2

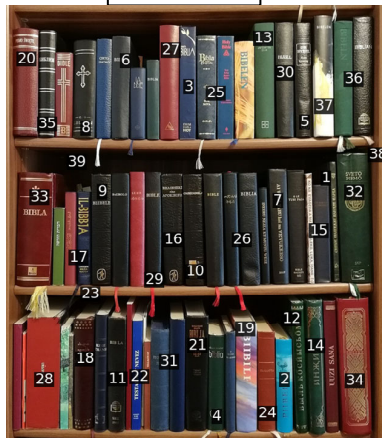

Level - 3

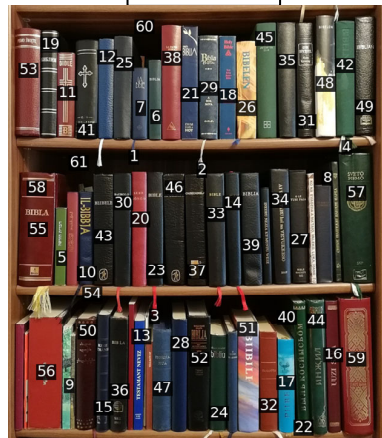

# SoM Granularity

Level - 1

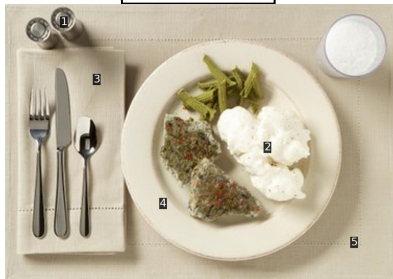

Level - 2

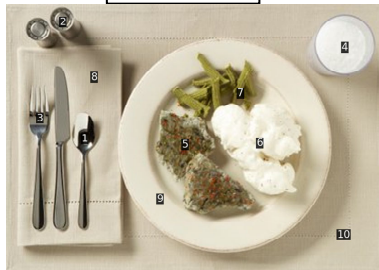

Level - 3

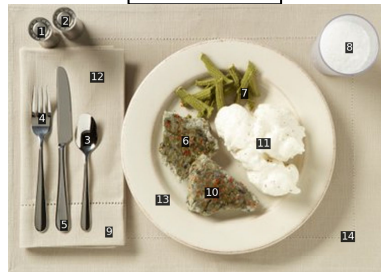

# SoM Granularity

Level - 1

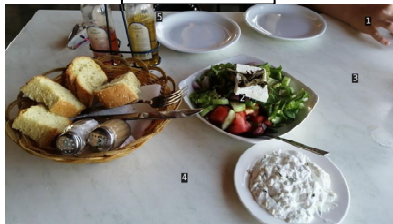

Level - 2

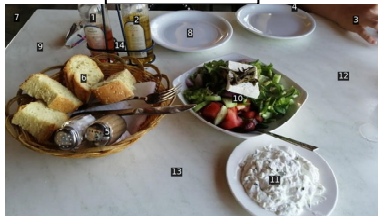

Level - 3

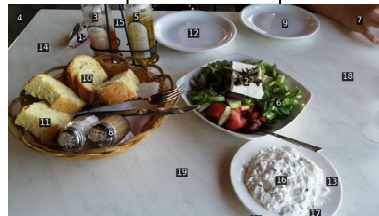

## SoM Granularity

Level - 1

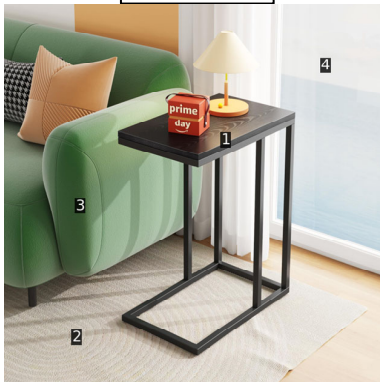

Level - 2

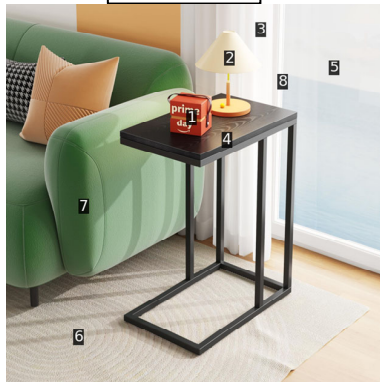

Level - 3

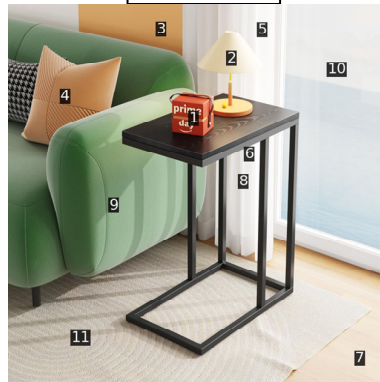

Supplement: Supplementary file 1 [file appendix.som.granularity.pdf]
